# Supplementary material for: EmbodiedVSR: Dynamic Scene Graph-Guided Chain-of-Thought Reasoning for Visual Spatial Tasks
Source: arXiv:2503.11089 source file (2025-03-14)
Supplement: Supplementary file 1 [file appendix.tex]

\section{Appendix}
